# Supplementary material for: Coarse-graining dynamics to maximize irreversibility
Source: arXiv:2506.01909 ancillary file (2025-06-02)
Supplement: Supplementary file 1 [file si.pdf]

# Supplemental Material: Coarse-graining dynamics to maximize irreversibility

Qiwei Yu,[1] Matthew P. Leighton,[2] and Christopher W. Lynn[2,3]

[1]Lewis-Sigler Institute for Integrative Genomics, Princeton University, Princeton, NJ 08544
[2]Department of Physics and Quantitative Biology Institute, Yale University, New Haven, CT 06511
[3]Wu Tsai Institute, Yale University, New Haven, CT 06510

## CONTENTS

I. Additional theoretical details S1
A. Proof for $\Delta\sigma \geq 0$ S1

II. Numerical details for examples in the main text S2
A. Kinesin motor S2
B. Brusselator S2
C. Neural activities in the mouse hippocampus S3
1. Definition of irreversibility S3
2. Max correlation coarse-graining S4
3. Positional information in neural activities S4
4. Place and non-place cells in coarse-grained neurons S5
5. Robustness of the results S6

References S6

## I. ADDITIONAL THEORETICAL DETAILS

### A. Proof for $\Delta\sigma \geq 0$

Here, we show explicitly that coarse-graining does not increase the irreversibility $\sigma$ as defined in the main text. The decrease in irreversibility is given by

$$\Delta\sigma = \frac{1}{2}\left[\sum_{i,j}\hat{\sigma}(J_{ij}, J_{ji}) - \sum_{\alpha,\beta}\hat{\sigma}(J_{\alpha\beta}, J_{\beta\alpha})\right] \tag{S1}$$

$$= \frac{1}{2}\sum_{\alpha,\beta}\left[\sum_{i\in\alpha,j\in\beta}\hat{\sigma}(J_{ij}, J_{ji}) - \hat{\sigma}(J_{\alpha\beta}, J_{\beta\alpha})\right] \tag{S2}$$

$$= \frac{1}{2}\sum_{\alpha,\beta}\left[\sum_{i\in\alpha,j\in\beta}\hat{\sigma}(J_{ij}, J_{ji}) - \hat{\sigma}\left(\sum_{i\in\alpha,j\in\beta}J_{ij}, \sum_{i\in\alpha,j\in\beta}J_{ji}\right)\right] \equiv \frac{1}{2}\sum_{\alpha,\beta}\Delta\sigma_{\alpha\beta}. \tag{S3}$$

Thus, it suffices to show that $\Delta\sigma_{\alpha\beta} \geq 0$ for all pairs of coarse-grained states $\alpha$ and $\beta$. This follows from Jensen's inequality: since $f(t) \equiv \hat{\sigma}(t, 1) = (t-1)\ln t$ is a convex function for $t > 0$, we have for $\mu_i > 0$ and $t_i > 0$

$$\sum_k \mu_k f(t_k) \geq f\Big(\sum \mu_k t_k\Big). \tag{S4}$$

Substituting $t_k = J_{ij}/J_{ji}$ and $\mu_k = J_{ji}/J_{\beta\alpha}$ where $k$ enumerates all pairs of $i \in \alpha$ and $j \in \beta$, we have

$$\sum_{i\in\alpha,j\in\beta}\frac{J_{ji}}{J_{\beta\alpha}}f\left(\frac{J_{ij}}{J_{ji}}\right) \geq f\left(\sum_{i\in\alpha,j\in\beta}J_{ij}/J_{\beta\alpha}\right) = f\left(\frac{J_{\alpha\beta}}{J_{\beta\alpha}}\right). \tag{S5}$$

Multiplying both sides by $J_{\beta\alpha}$, we have

$$\sum_{i\in\alpha,j\in\beta}\hat{\sigma}(J_{ij},J_{ji})=\sum_{i\in\alpha,j\in\beta}J_{ji}f\left(\frac{J_{ij}}{J_{ji}}\right)\geq J_{\beta\alpha}f\left(\frac{J_{\alpha\beta}}{J_{\beta\alpha}}\right)=\hat{\sigma}(J_{\alpha\beta},J_{\beta\alpha}), \tag{S6}$$

which proves that $\Delta\sigma_{\alpha\beta}\geq 0$ for all pairs of coarse-grained states $\alpha$ and $\beta$ and thus $\Delta\sigma\geq 0$.

## II. NUMERICAL DETAILS FOR EXAMPLES IN THE MAIN TEXT

### A. Kinesin motor

Here, we study two discrete-state models for the mechanochemical cycle of the kinesin-1 motor protein. The first is the four-state model proposed in Ref. [1]. We use the reported rate constants from fits to experimental data, with zero load (external force $F=0$) and ATP concentration $c_{\text{ATP}}=1000\mu$M.

The second model we consider is the 6-state model proposed in Ref. [2], with the reported rate constants from fits to experimental data [3]. For consistency with the 4-state model, we use zero load (external force $F=0$), and concentrations of ATP, ADP, and inorganic phosphate given by $c_{\text{ATP}}=1000\mu$M, $c_{\text{ADP}}=0.5\mu$M, and $c_{\text{P}_\text{i}}=0.5\mu$M.

For both models, we solve the master equation numerically to obtain steady state probabilities and fluxes. The net fluxes between pairs of states are illustrated in Figs. 1a and 1c, where arrow thickness scales with net flux. The flux arrows are colored to denote the nature of the transition; transitions between states arise from binding/unbinding of ATP, ADP, and $\text{P}_i$, as well as ATP hydrolysis.

For both models, we enumerate all possible CGs, and compute and plot the irreversibility in Figs. 1b and 1e respectively. In Fig. 1e the optimal CG is obtained either via the greedy CG procedure, or by selecting the maximal irreversibility over all possible CGs. The "random" curve is computed by averaging over all possible CGs.

Figure 1d shows the optimal four-state CG for the 6-state model. This is achieved by combining states 1 and 6, and states 4 and 5; combining these states in either order leads to the same coarse-grained model.

### B. Brusselator

Here, we study the simplified Brusselator model [4–6], which describes the dynamics of two chemical species $X$ and $Y$ with reactions

$$A\underset{k_{-1}}{\overset{k_1}{\rightleftharpoons}}X,\qquad B\underset{k_{-2}}{\overset{k_2}{\rightleftharpoons}}Y,\qquad 2X+Y\underset{k_{-3}}{\overset{k_3}{\rightleftharpoons}}3X, \tag{S7}$$

with $k_{\pm i}$ being kinetic constants of each reaction $\pm i$, and $A$ and $B$ molecules held at constant concentrations. We assume mass-action kinetics, where the transition rates are given by the product of kinetic constants and the concentrations of the substrate; for instance, the forward rate of reaction 3 is $k_3[X]^2[Y]$, with concentrations $[X]=N_X/V$ and $[Y]=N_Y/V$. We use the following parameter values: $k_1=5$, $k_{-1}=15$, $k_2=15$, $k_{-2}=0.5$, $k_3=2$, $k_{-3}=1$, and the volume is $V=9$.

The state space is a 2-dimensional lattice spanned by $\boldsymbol{n}=(N_X,N_Y)$ (see Fig. 2a of the main text), with local transitions representing the three reactions above. The steady-state probability $P(N_X,N_Y)$ and probability fluxes are determined by solving the chemical master equation for $N_X\in[0,80]$ and $N_Y\in[0,160]$. For better visualization, the flux in Fig. 2(a) was averaged over $8\times 8$ neighborhoods.

In the main text, Fig. 2(c) visualizes the fluxes between coarse-grained states by plotting a heatmap of $J_{i,j}=\sqrt{J_{i,j,X}^2\delta_{i,j,X}+J_{i,j,Y}^2\delta_{i,j,Y}}$, where $J_{i,j,X}$ and $J_{i,j,Y}$ are the fluxes in the $X$ and $Y$ directions, respectively. $\delta_{i,j,X}=1$ if states $(i,j)$ and $(i+1,j)$ belong to different coarse-grained states, and $\delta_{i,j,X}=0$ otherwise. Similarly, $\delta_{i,j,Y}=0,1$ indicates whether states $(i,j)$ and $(i,j+1)$ belong to different coarse-grained states. Therefore, this definition ensures that fluxes within a coarse-grained state are not shown, and only those between coarse-grained states are captured. These definitions are for visualization purposes only and do not affect the coarse-graining procedure.

For comparison, Fig. S1 shows the fluxes for random and square blocking coarse-graining, which do not capture the limit cycle structure as well as the optimal coarse-graining procedure [Fig. 2(c) in the main text].

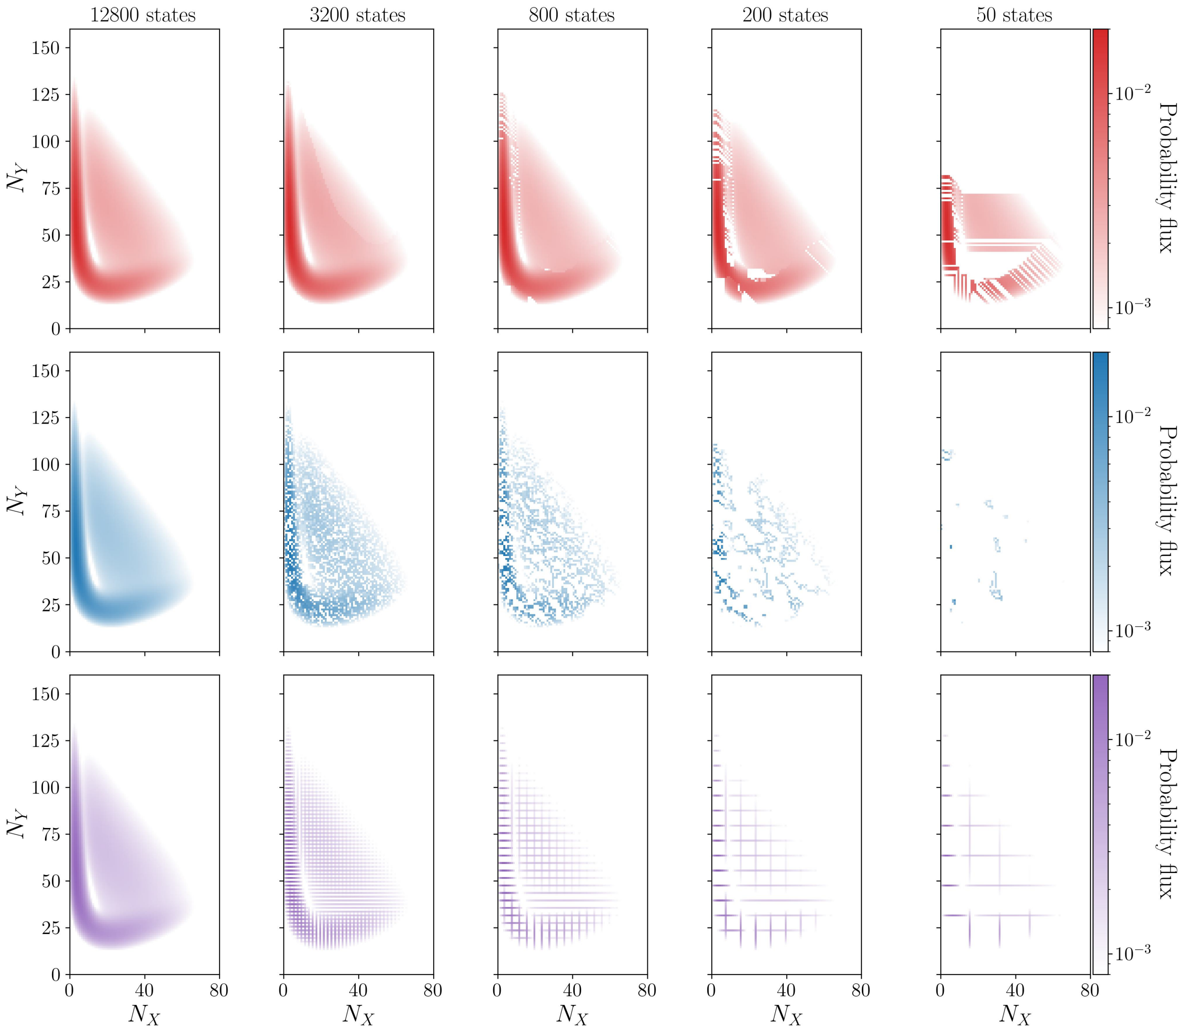


FIG. S1. Net fluxes between states for different coarse-graining procedures (rows) and different levels of coarse-graining (columns). The colors indicate the coarse-graining procedure: top (red): optimal CG; middle (blue): random CG; bottom (purple): square blocking. Each column is a level of coarse-graining, with the leftmost column being the original state space. Note that fluxes within each coarse-grained states are no longer visible.

## C. Neural activities in the mouse hippocampus

### 1. *Definition of irreversibility*

Neural activities in the mouse hippocampus were measured as it runs along a virtual track [7]. The activity of $N = 1485$ neurons was recorded using two-photon calcium imaging with a sampling frequency of $f = 30$Hz. The activities are binarized, i.e., $a_i(t) = 0, 1$ for the activity of neuron $i$ at time $t$. To describe the neural activities with a stochastic jump process, we define the state of the population $n(t)$ as the most recent neuron firing at time $t$. Thus, we arrive at a system with $N$ states, one for each neuron.

State transitions are defined by pairs of neurons that are active at time $t$ and $t + \Delta t$. The probability flux $J_{n \to n'}$ thus describes the flow of activities from neuron $n$ to neuron $n'$. We extract it from the measurements by counting the average number of transitions from state $n$ to $n'$ per unit time

$$J_{ij} = \frac{1}{T - \Delta t} \sum_{t=0}^{T-\Delta t} j_{ij}(t, t + \Delta t) = \frac{1}{T - \Delta t} \sum_{t=0}^{T-\Delta t} w(t, t + \Delta t) a_i(t) a_j(t + \Delta t), \tag{S8}$$

where $\Delta t$ is a time delay, and $T$ is the total time of the measurement. In the main text, we set $\Delta t = 3$s, but none of

the main results are sensitive to the choice of $\Delta t$ (see Sec. II C 5).

The weight $w(t, t+\Delta t)$ is introduced to account for the fact that multiple neurons can be active within the time resolution of the measurement $f^{-1} = 1/30\text{s}$. Therefore, we need to average the probability flux over all possible dynamics that are consistent with the observed activities. This leads to $w(t, t+\Delta t) = \frac{1}{A(t)A(t+\Delta t)}$, where $A(t) = \sum_{i=1}^{N} a_i(t)$ is total activity at time $t$. This definition ensures that Kirchhoff's first law is satisfied, i.e., the total flux into a state equals the total flux out of it, since each active neuron will receive the same amount of incoming and outgoing flux at a given time:

$$\sum_j j_{ij}(t, t+\Delta t) = a_i(t) \sum_j w(t, t+\Delta t) a_j(t+\Delta t) \tag{S9}$$

$$= \sum_j j_{ji}(t-\Delta t, t) = a_i(t) \sum_j w(t-\Delta t, t) a_j(t-\Delta t) \tag{S10}$$

$$= \frac{a_i(t)}{A(t)} \tag{S11}$$

where the first line is the outgoing flux from state $i$ at time $t$, and the second line is the incoming flux to state $i$ at time $t$. The total flux in the system is invariant over time:

$$\sum_{ij} j_{ij}(t, t+\Delta t) = \sum_i \frac{a_i(t)}{A(t)} = 1. \tag{S12}$$

The local irreversibility is defined as

$$\sigma = \sum_{ij} (J_{ij} - J_{ji}) \ln \frac{J_{ij} + \epsilon}{J_{ji} + \epsilon}, \tag{S13}$$

where a small number $\epsilon$ ensures that the logarithm is well-defined. We set $\epsilon = 1/(T - \Delta t)$, but the results are not sensitive to this choice. Note that we can still define irreversibility $\sigma$ even though the stochastic jump process is not Markovian. With irreversibility defined, coarse-graining can be carried out following the procedure described in the main text.

### 2. *Max correlation coarse-graining*

For max correlation coarse-graining, we first compute the correlation coefficient between the activities of all pairs of neurons

$$C_{ij} = \frac{\langle \delta a_i(t) \delta a_j(t) \rangle}{\sqrt{\langle (\delta a_i(t))^2 \rangle \langle (\delta a_j(t))^2 \rangle}}, \tag{S14}$$

where $\delta a_i(t) = a_i(t) - \langle a_i(t) \rangle$ is the deviation of the activity of neuron $i$ from its average, and $\langle \cdots \rangle$ is the average over time. Then we pick the pair of states with the largest correlation coefficient $C_{ij}$, and combine them to form a new state $\alpha$ with activity $a_\alpha(t) = F[a_i(t), a_j(t)]$. $F$ follows the majority rule of block spin transformation of the Ising model: If the two states are both active (inactive) at time $t$, then the new state is active (inactive) at time $t$; otherwise, if $i$ and $j$ have opposite activities, the new state $\alpha$ is assigned to be inactive (active) at time $t$ with probability $p = 1/2$. This process is repeated until the desired number of coarse-grained states is reached.

### 3. *Positional information in neural activities*

The experiment also measured the position of the mouse along the virtual track $x(t)$ [7], which allows us to compute the average firing rate of each neuron $i$ for each position $x$:

$$\tilde{a}_i(x) = \frac{\sum_t a_i(t) \delta(x(t) - x)}{f^{-1} \sum_t \delta(x(t) - x)}, \tag{S15}$$

where $t$ sums over discrete time points. The numerator is the total number of spikes of neuron $i$ at position $x$, and the denominator is the total time spent at position $x$, with $f = 30\text{Hz}$ being the sampling frequency. For coarse-grained

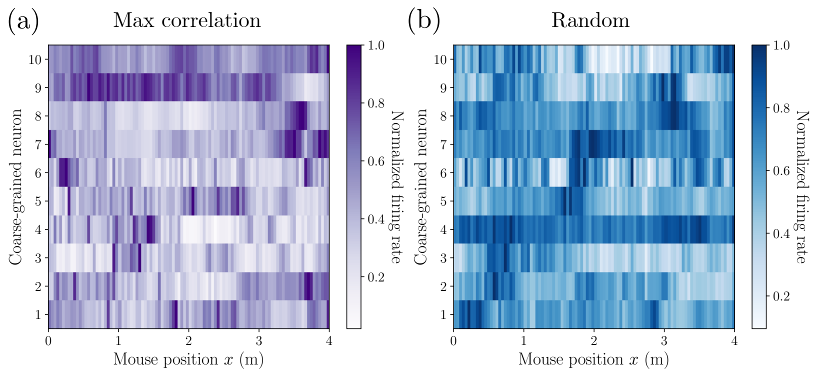


FIG. S2. Place field of coarse-grained neurons due to maximum correlation CG (a) and random CG (b).

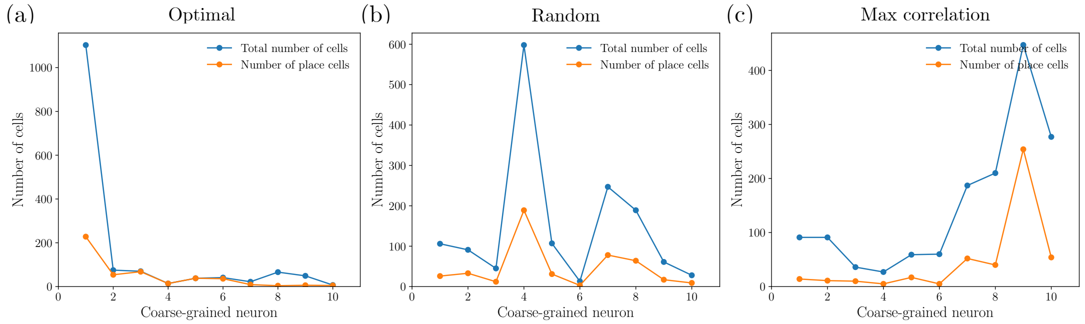


FIG. S3. The composition of the macrostates due to 10-state coarse-graining. The method for identifying place cells is detailed in Ref. [8].

neurons, the firing rate is given by the sum of the activities of all constituent neurons, $\tilde{a}_\alpha(x) = \sum_{i\in\alpha} \tilde{a}_i(x)$, where $\alpha$ is the index of the coarse-grained neuron.

We can compare the firing patterns of neurons due to optimal CG (Fig. 3c, bottom panel) with those due to random and max correlation CG procedures (Fig. S2), which do not show a clear spatial structure.

For a set of neurons with the firing pattern $\{\tilde{a}_\alpha(x)\}$, the joint probability distribution $P(x,\alpha)$ for an observed spike to come from neuron $\alpha$ when the mouse is at position $x$ is given by

$$P(x,\alpha) = \frac{P_m(x)\tilde{a_\alpha}(x)}{\sum_\alpha \int \mathrm{d}x\, P_m(x)\tilde{a_\alpha}(x)}, \tag{S16}$$

where $P_m(x)$ is the probability of finding the mouse at position $x$. Note that $P_m(x)$ is different from the marginal probability $P(x) = \sum_\alpha P(x,\alpha) \neq P_m(x)$, since the total firing rate $\sum_\alpha \tilde{a}_\alpha(x)$ is not uniform in space.

To quantify how well neural activities represent spatial information, we ask how much information about the position $x$ can be inferred from observing a spike of neuron $\alpha$. This is given by the mutual information between the position $x$ and neuron identity $\alpha$

$$I(x,\alpha) = \int \mathrm{d}x \sum_\alpha P(x,\alpha) \ln \frac{P(x,\alpha)}{P(x)P(\alpha)} = \int \mathrm{d}x \sum_\alpha P(x,\alpha) \ln \frac{P(x|\alpha)}{P(x)} = H(x) - H(x|\alpha). \tag{S17}$$

For the results in Fig. 3(d) in the main text, we choose $P_m(x)$ to be uniform, i.e., $P_m(x) = 1/L$ with $L$ being the length of the track. The mutual information involves a spatial integral, which is computed by discretizing the position $x$ into bins of size $\Delta x$ and extrapolating the mutual information to $\Delta x \to 0$.

#### *4. Place and non-place cells in coarse-grained neurons*

Fig. S3 shows the composition of the macrostates due to 10-state coarse-graining. Place cells were identified using the approach detailed in Ref. [8]. For optimal coarse-graining, most of the non-place cells are grouped into the first macro-cell, which exhibits uniform activity along the track [Fig. 3(c) in the main text].

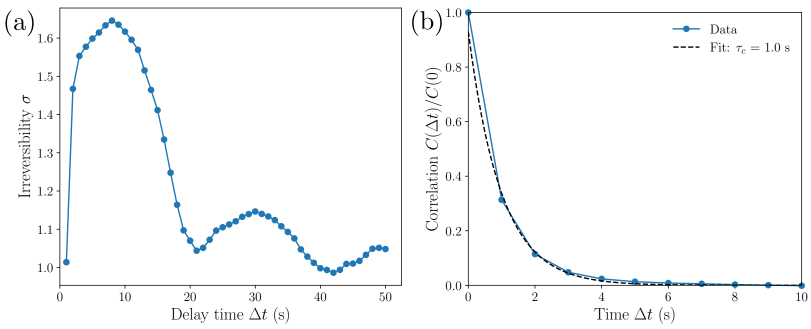


FIG. S4. Irreversibility and correlation as a function of delay time $\Delta t$.

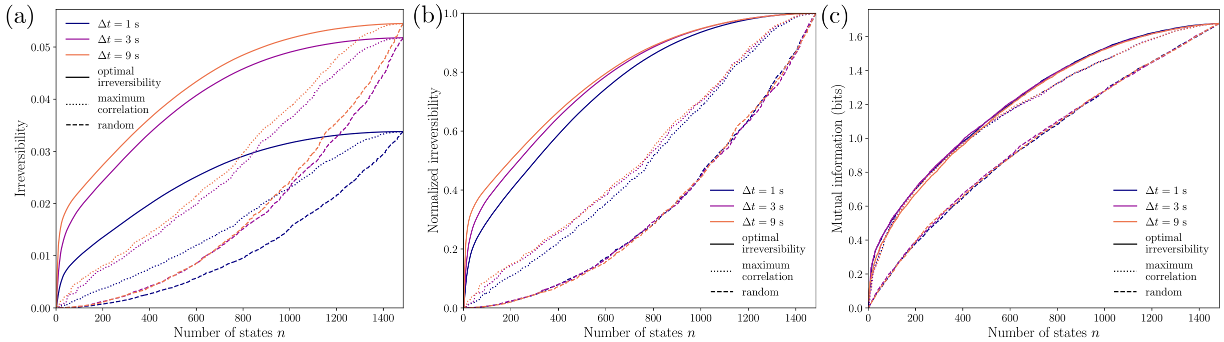


FIG. S5. The coarse-graining results are robust to the choice of delay time $\Delta t$. (a) The absolute value of the local irreversibility $\sigma$ as a function of the delay time $\Delta t$. (b) The fraction of irreversibility captured by the coarse-grained neurons as a function of $\Delta t$. (c) The amount of positional information in the coarse-grained neurons as a function of $\Delta t$.

### 5. *Robustness of the results*

Our definition of the probability flux $J_{ij}$ depends on the choice of delay time $\Delta t$. The main text focused on coarse-graining with a particular delay time $\Delta t = 3$s. This is motivated by the correlation structure and total irreversibility in the data (Fig. S4). $\Delta t = 3$s is comparable to the correlation time $\tau_c = 1$s and also captures a large amount of irreversibility. However, it should be noted that although varying $\Delta t$ affects the amount of local irreversibility $\sigma$ in the data, but it does not affect the main results, including the fraction of irreversibility captured due to coarse-graining, and the amount of positional information in the coarse-grained neural activities (Fig. S5). Therefore, any reasonable choice of $\Delta t$ will lead to the same conclusion.

## REFERENCES

[1] M. E. Fisher and A. B. Kolomeisky, Simple mechanochemistry describes the dynamics of kinesin molecules, Proceedings of the National Academy of Sciences **98**, 7748 (2001).
[2] S. Liepelt and R. Lipowsky, Kinesin's network of chemomechanical motor cycles, Physical review letters **98**, 258102 (2007).
[3] N. J. Carter and R. Cross, Mechanics of the kinesin step, Nature **435**, 308 (2005).
[4] G. Nicolis and I. Prigogine, *Self-organization in non-equilibrium systems* (Wiley, New York, 1997).
[5] J. H. Fritz, B. Nguyen, and U. Seifert, Stochastic thermodynamics of chemical reactions coupled to finite reservoirs: A case study for the brusselator, J. Chem. Phys. **152**, 235101 (2020).
[6] Q. Yu and P. E. Harunari, Dissipation at limited resolutions: power law and detection of hidden dissipative scales, J. Stat. Mech. **2024**, 103201 (2024).
[7] J. L. Gauthier and D. W. Tank, A dedicated population for reward coding in the hippocampus, Neuron **99**, 179 (2018).
[8] K. Shi and C. W. Lynn, Neural flow in the hippocampus reveals timescales in behavior, *in prep.*
